# Supplementary material for: Full control of solid-state electrolytes for electrostatic gating
Source: arXiv:2302.11967 ancillary file (2023-02-23)
Supplement: Supplementary file 1 [file SI_Fullcontrolof_CAO.pdf]

# Supporting information for Full control of solid-state electrolytes for electrostatic gating

Chuanwu Cao<sup>1,2</sup>, Margherita Melegari<sup>1,2</sup>, Marc Philippt<sup>1,2</sup>, Daniil Domaretskiy<sup>1,2</sup>, Nicolas Ubrig<sup>1,2</sup>, Ignacio Gutiérrez-Lezama<sup>1,2</sup>, and Alberto F. Morpurgo<sup>1,2</sup>\*

<sup>1</sup> Department of Quantum Matter Physics, University of Geneva, 24 Quai Ernest Ansermet, Geneva CH-1211, Switzerland

<sup>2</sup> Department of Applied Physics, University of Geneva, 24 Quai Ernest Ansermet, Geneva CH-1211, Switzerland

\*Email Address: alberto.morpurgo@unige.ch

## S1. Stability of LICGC-gated FETs without a SiO<sub>2</sub> passivation layer

In the main text we show that –in the absence of a passivation layer between the Li-ion conducting glass-ceramic (LICGC) substrate and the Pt contacts of the field-effect transistors (FETs)– electrochemical reactions occur and result in the absence of electron accumulation, as well as other spurious effects (see Figs. 2c-f) at positive gate voltages. In this section we demonstrate that these electrochemical reactions do not cause an irreversible degradation of the LICGC-gated devices. To this end, Fig. S1 shows the transfer curves measured on a transistor several days apart, period during which the device was used to do a variety of different measurements. As it is apparent from the data, despite the application of positive gate voltages for an extended period of time, the dependence of the current  $I_{SD}$  on gate voltage  $V_G$  remains virtually unchanged (except for a small threshold voltage shift for hole accumulation, due to common bias stress effects).

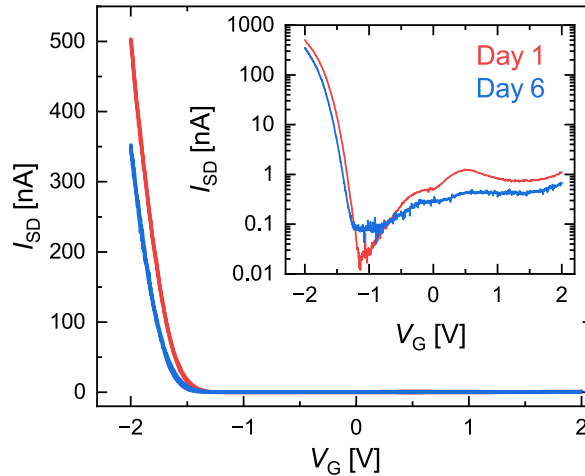

Figure S1: Source-drain current  $I_{SD}$  versus applied gate voltage  $V_G$  in a LICGC-gated FET based on a thick exfoliated WSe<sub>2</sub> crystal, with no SiO<sub>2</sub> passivation layer. Measurements performed 6 days apart after continuous sweeping of the gate voltage to positive and negative values show the same response of  $I_{SD}$  to  $V_G$ . The small threshold voltage shift observed between the two curves is the result of bias stress effects, difficult to avoid when operating ionic gated devices for very extended periods of time. The similarity between the two measurements is also evident when plotting the data in semi-log scale, as shown in the inset.

## S2. Extended cyclic voltammetry data

In the main text we discuss the results of cyclic voltammetry (CV) measurements performed on two-terminal ionic liquid and LICGC devices, which we employ to detect the presence of electrochemical reactions at the LICGC/Pt interface and to determine how to prevent their impact on the performance of

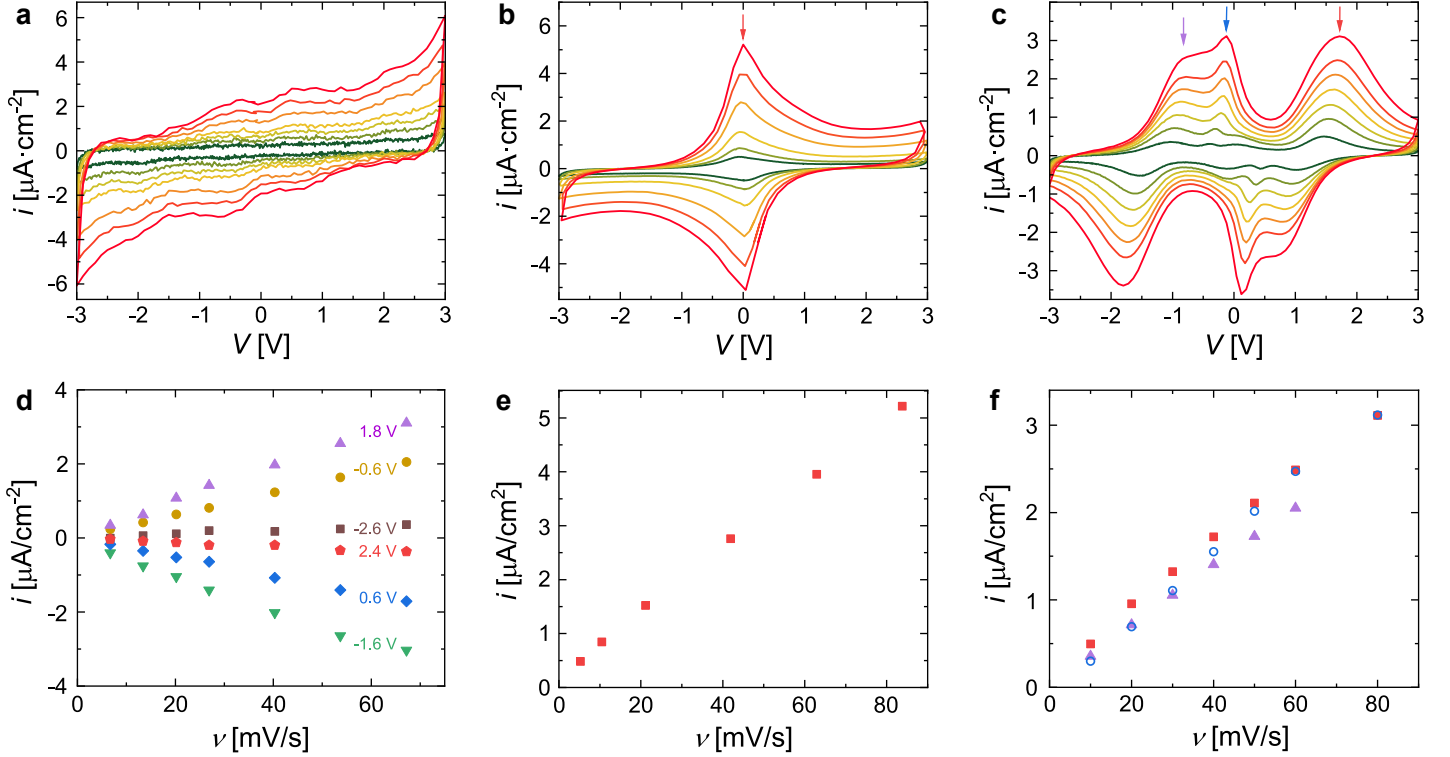

Figure S2: CV measurements performed on two-terminal ionic liquid and LICGC devices. Current density  $i$  (current  $I$  divided by the geometrical area of the electrode) vs voltage  $V$  measured in **a)** Au/ionic-liquid/Au (same as in Fig. 3a), **b)** Pt/LICGC/Pt (same as in Fig. 3b) and **c)** Cr/LICGC/Cr devices (from the green to the red curves the sweep rate  $\nu$  values are 7, 13, 20, 27, 40, 54 and 67 mV/s in a), 5, 10, 21, 42, 63 and 84 mV/s in b) and 10, 20, 30, 40, 50, 60 and 80 mV/s in c)). The geometrical area of the Au and the Pt electrodes in a) and b) is  $700\ \mu\text{m} \times 700\ \mu\text{m}$ , and that of the Cr electrodes in c) is  $500\ \mu\text{m} \times 500\ \mu\text{m}$ . The dependence of  $i$  on  $\nu$  for selected voltage values in a) and for the voltages tracing the evolution of the peaks indicated by the arrows in b) and c) are shown in **d)**, **e)** and **f)**, respectively. All the panels show a linear evolution of  $i$  on  $\nu$ .

LICGC-gated FETs (see Fig. 3). In this section we provide additional information regarding several aspects of the CV data that are mentioned in the main text.

We start by showing in Fig. S2d the dependence of the current density  $i$  on sweep rate  $\nu$  in Au/ionic-liquid/Au devices (known as CV-IL devices; for convenience, in Fig. S2a we reproduce the CV data shown in Fig. 3a in terms of  $i$ ). As mentioned in the main text,  $i$  follows a linear dependence on  $\nu$  and extrapolates to zero within the sensitivity of our measurements, as  $\nu$  vanishes, as expected for the charging of and electric double layer (EDL).

The discussion in the main text centers around CV measurements performed on LICGC devices contacted with Pt electrodes because Pt is systematically used to make good contact with few-layer transition-metal dichalcogenide (TMD) semiconductors (such as  $\text{WSe}_2$ ). In this section we also show that electrochemical reactions take place at the interface between the LICGCs and other metals. As an example, we discuss CV measurements performed on Cr/LICGC/Cr devices, but we note that electrochemical reactions also occur at the interface with a variety of other metals, such as Ti and Ag.

Fig. S2 shows a comparison between the results of CV measurements performed on Pt/LICGC/Pt (Figs. S2b and e) and Cr/LICGC/Cr (Figs. S2c and f) devices for multiple sweep rates. For the Pt electrode device, a peak centered around 0 V is seen in the  $i$ -vs- $V$ -curves for both the anodic and cathodic sweeps, signaling the presence of a single electrochemical reaction [1–3] (Fig. S2b). In turn, in the Cr electrode device three peaks are present at around  $\approx -1$  V,  $\approx -0.25$  V and  $\approx 1.5$  V in the anodic sweep (at

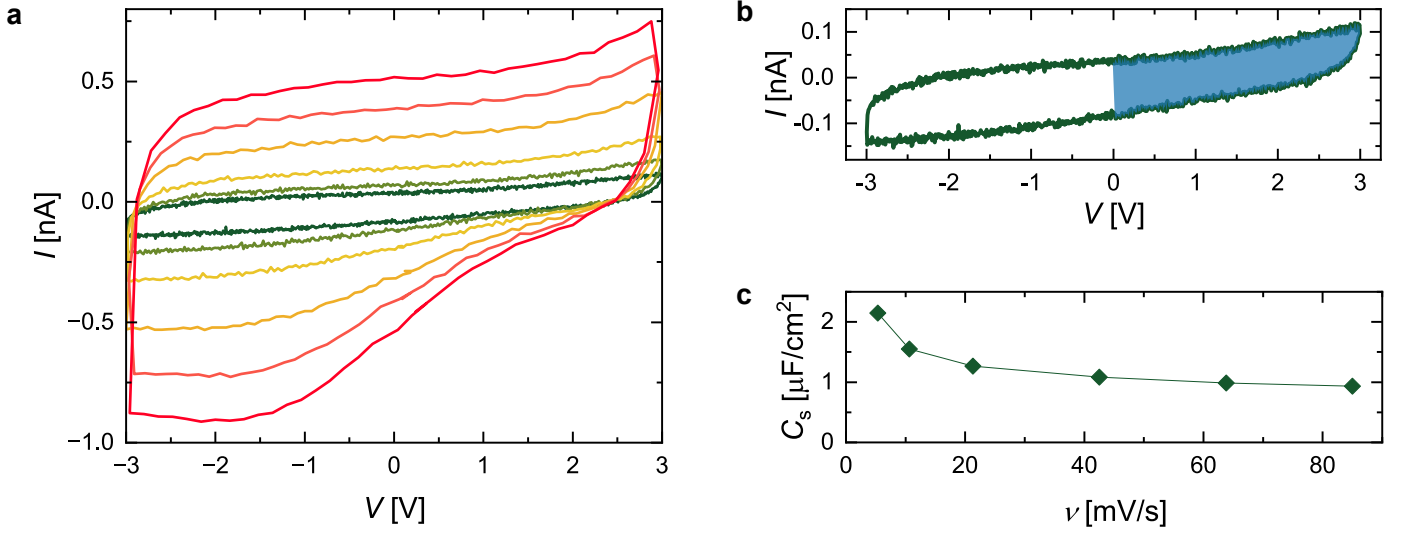

Figure S3: CV measurements performed on a two-terminal device where a  $\text{SiO}_2$  passivation layer is placed in between one of the Pt electrodes and the LICGC (see Fig. 3c for device schematics). **a)** CV curves at different sweep rates (from the green to the red curve the sweep rates are 5, 11, 21, 43, 64 and 85 mV/s). **b)** For all different sweeping rate, the area delimited by the CV curve –shaded in blue in this example– is used to extract the value of the capacitance plotted in panel c) and in Fig. 3d. What determines the extent of the shaded area is the in-series connection of the capacitance of the LICGC/Pt and LICGC/ $\text{SiO}_2$ /Pt interface, when the applied voltage pushes Li ions towards the LICGC/ $\text{SiO}_2$ /Pt interface. The asymmetry of the CV curves shown in a) and b) originates from the fact that (irrespective of the metal used) the double layer capacitance is different upon accumulation or depletion of Li-ions. **c)** In-series geometrical capacitance per unit area  $C_s$  plotted as a function of sweep rate, extracted from the CV curves shown in panel a) by calculating the enclosed area (as illustrated in panel b)).

the highest sweep rate) and occur in reverse order in the cathodic sweep (e.g., the peak seen at  $-1$  V in the anodic sweep is present at  $1$  V in the cathodic sweep, etc; Fig. S2f). We note that a fourth peak is present at low sweep rates at  $\approx 0$  V for both sweep directions but it is quickly eclipsed by the peak seen at  $\approx -0.25$  V at higher sweep rates). The multiple peak structure signals the presence of multiple reactions revealing a more complex interfacial chemistry [1–3].

As discussed in the main text, the peaks are created by faradaic reactions of the type  $x\text{Li}^+ + xe^- + \text{R} \rightleftharpoons \text{Li}_x\text{R}$  (R is the reduced species), taking place at the electrolyte/electrode interface, whose reaction dynamics is controlled by the formation of a self-limiting Nernstian diffusion layer and by the electroadsorption of species resulting in a pseudocapacitive contribution to the current [1–3]. Finding that the peak current has a linear dependence on sweep rate  $\nu$  [1–3], as shown in Figs. S2e and f for both devices, confirms that pseudocapacitive effects are present at the LICGC/metal interface. For both metals the most likely origin of the pseudocapacitance is the intercalation of Li in the  $\text{TiO}_2$  [4], which has been reported for similar glass-ceramics [5, 6], with the multiple peaks in the Cr device arising from intermediate reactions due to its higher reactivity. Elucidating the exact origin of the electrochemical reactions would require a detail investigation that is out of the scope of this work. Our purpose is to identify the presence of reactions so that their negative effect on the operation of transistors can be prevented.

Finally, we discuss CV measurements performed on Pt/LICGC/ $\text{SiO}_2$ /Pt devices. As stated in the main text, placing a  $\text{SiO}_2$  passivation layer between the LICGC and the Pt electrodes results in the absence of the faradaic current peaks (see Fig. S3a) caused by the electrochemical reactions taking place between the ceramic substrate and the Pt electrodes (see Fig. S2b), a solution we employ to realize properly working LICGC-gated FETs. Figs. S3a and c (see also Figs. 3c and d) however show that the displacement current present in the Pt/LICGC/ $\text{SiO}_2$ /Pt device and the corresponding extracted capacitance are larger than expected for a 40 nm  $\text{SiO}_2$  layer, providing some insight regarding the mechanism that prevents electrochemical reactions from taking place. Given the large capacitance, which is more reminiscent of

sub nano-gap capacitors, we conclude that Li ions can migrate within the  $\text{SiO}_2$  layer (despite the high quality of e-beam evaporated  $\text{SiO}_2$  (could be  $\text{SiO}_x$  due to defects formed during the evaporation), which has similar insulating properties to thermally grown  $\text{SiO}_2$  [7]). From this observation, we infer that the role of the  $\text{SiO}_2$  likely is to act as a passivation layer that physically separates the  $\text{TiO}_2$  present in the LICGC from the electrons in the Pt contact, preventing the formation of  $\text{Li}_x\text{TiO}_2$ , as mentioned in the main text.

### S3. Influence of the LICGC/Pt contact area on the electrical characteristics of LICGC-gated FETs

In the main text we show that electrochemical reactions at the LICGC/Pt interface prevent the correct operation of LICGC-gated FETs for positive gate voltage ( $V_G$ ), resulting in the absence of electron transport, the saturation of the reference potential  $V_{\text{Ref}}$  and the concomitant appearance of peaks in the leakage current  $I_G$  (see Figs. S4a-c and Figs. 2c-f). We also demonstrate that high-quality ambipolar LICGC-gated FETs are realized when these parasitic effects are avoided by placing a  $\text{SiO}_2$  passivation layer between the LICGC and the Pt electrodes (see Figs. S4j-l and Figs. 4a-c). Here we focus on the evolution of the electrical characteristics of FETs with decreasing LICGC/Pt interfacial contact area, which gives further insight into the mechanism that prevents correct FET operation in the presence of electrochemical reactions.

Figs. S4d-f show that placing a passivation layer in between a large portion of the LICGC/Pt interface (reducing the LICGC/Pt contact area from  $\approx 10^5 \mu\text{m}^2$  in devices without  $\text{SiO}_2$  to  $\approx 10^4 \mu\text{m}^2$ ) results in a partial improvement of the performance of the FETs. In this device electron transport is present, the saturation of  $V_{\text{Ref}}$  is seen over a smaller  $V_G$  interval, and disappears at sufficiently large  $V_G$ , and the  $I_G$  peaks caused by the electrochemical reactions (labeled A and B) decrease in magnitude. Further improvement, resulting in almost parasitic-free transistor characteristics (Figs. S4g-i), is achieved when the LICGC/Pt contact area is reduced to a size comparable to that of the 2D crystal (from  $\approx 10^4 \mu\text{m}^2$  to  $\approx 10^3 \mu\text{m}^2$ ). In this case electron transport is present without the saturation of  $V_{\text{Ref}}$  that instead shows the expected linear dependence on  $V_G$ , and the  $I_G$  peaks (A and B) caused by the reactions decrease to a level allowing the observation of the peaks typically seen at the onset of charge accumulation (labeled C and D in Fig. S4i and l; see discussion in main text). Finally, completely suppressing the LICGC/Pt contact area results in the complete absence of the parasitic effects caused by electrochemical reactions (compare Figs. S4a-c to Figs. S4j-l).

The observed behaviour of  $I_G$  and  $V_{\text{Ref}}$  with decreasing LICGC/Pt contact area is consistent with the devices storing charge electrochemically instead of electrostatically (Ref. [8] provides a comprehensive discussing regarding the differences between the two storage mechanisms). As discussed in the main text, in the presence of chemical reactions the gate-electrode/LICGC/Pt structure behaves as a half cell [1, 3], whose cell potential is the gate voltage at which the  $I_G$  peaks are observed. Finding smaller  $I_G$  peak currents when the LICGC/Pt contact area is smaller is consistent with a lower capacity of the half cell; a smaller LICGC/Pt area results in a lower transfer of electrons, a lower current and a lower production of neutral species (note that the  $I_G$  peak current does not need to scale proportionally to the geometrical area of the LICGC/Pt interface because finite size effects can affect the effective area where the reaction takes place [9]). The amount of neutral species produced in each device is responsible for the different level of performance of each transistor. When a large amount of neutral species is generated (Figs. S4a-c), the presence of  $\text{Li}^+$  ions at the interface does not result in the accumulation of electrons for  $V_G$  values beyond the cell potential, leading to the saturation of  $V_{\text{Ref}}$  (see Fig. S4b). Because no additional potential is transferred to the device interface as  $V_G$  is increased, the gate loses its ability to control the chemical potential in the semiconductor and electron transport is not achieved (Fig. S4a). Instead, in devices where the full capacity of produced neutral species is reached (Figs. S4d-f),  $V_{\text{Ref}}$  recovers a linear dependence on  $V_G$  for voltages beyond the cell potential (see Fig. S4e), and electron transport is ob-

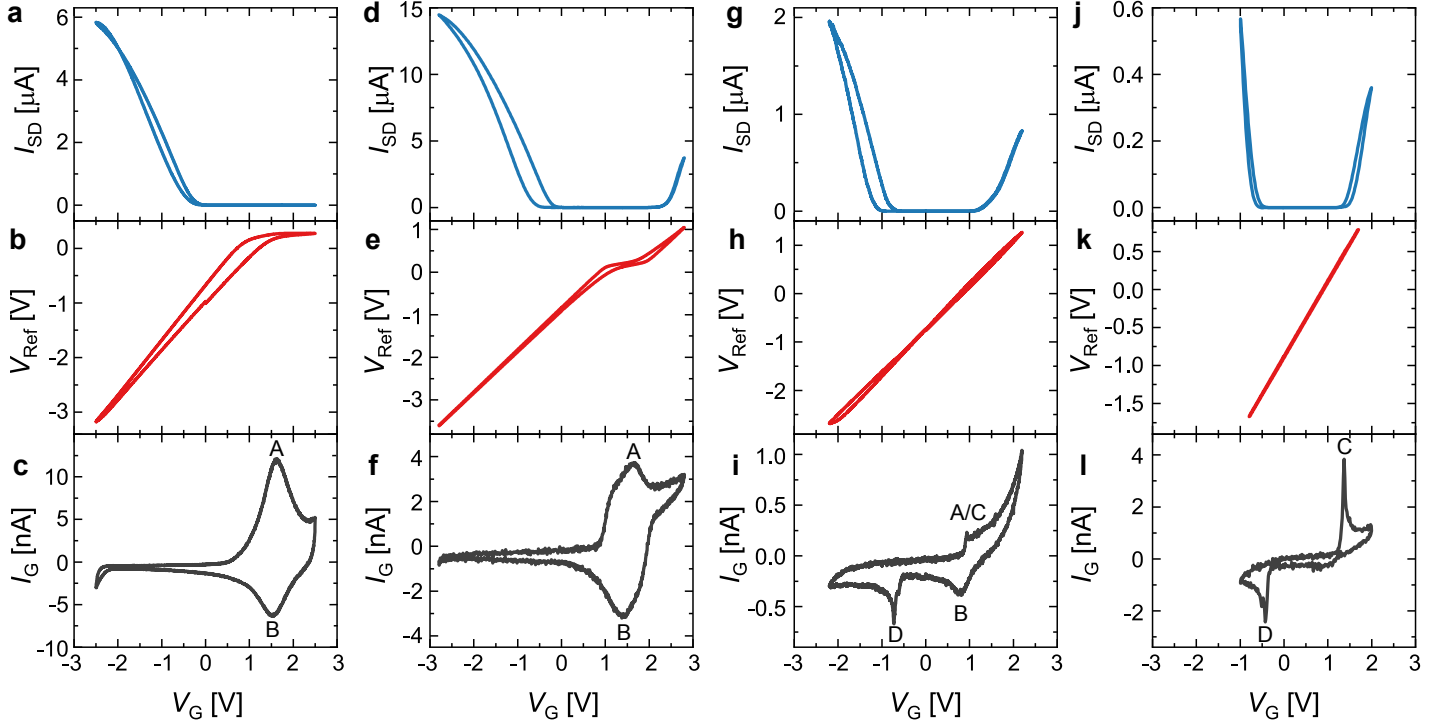

Figure S4: Comparison between the transistor characteristics of four WSe<sub>2</sub> LICGC-gated FETs with different LICGC/Pt contact areas. The LICGC/Pt contact area in a)-c), d)-f), g)-i) and j)-l) are  $4 \times 10^5 \mu\text{m}^2$  (same device as in Figs. 2c and d),  $1.5 \times 10^4 \mu\text{m}^2$ ,  $5 \times 10^3 \mu\text{m}^2$  and 0 (same device as in Figs. 4a and b), respectively. The transistor characteristics in a)-i) are measured on 3L-WSe<sub>2</sub> LICGC-gated FETs and those in j)-l) are on a 1L-WSe<sub>2</sub> LICGC-gated FET. **a), d), g) and j)** Source-drain current  $I_{\text{SD}}$ -vs-gate voltage  $V_{\text{G}}$  (transfer) curves ( $V_{\text{SD}} = 50 \text{ mV}$ ). **b), e), h) and k)** Response of the (non-local) reference potential  $V_{\text{Ref}}$  to  $V_{\text{G}}$ . **c), f), i) and l)** Response of the leakage current  $I_{\text{G}}$  to  $V_{\text{G}}$ . The sweep rates in a)-c), d)-f), g)-i) and j)-l) are 1.8 mV/s, 3 mV/s, 3 mV/s and 6.5 mV/s, respectively.

served because the gate regains its ability to control the chemical potential in the semiconductor (see Fig. S4d). In devices with a sufficiently small LICGC/Pt contact area the amount of neutral species that are produced are not sufficient to significantly affect the performance of the FETs (see Figs. S4g-i).

As a final remark we note that electron transport can be present in LICGC-gated FETs even in the absence of a passivation layer, as reported in recent work [10, 11]. This is possible when the threshold voltage for electrons is smaller than the gate voltage at which the reactions take place. However, in that case the onset of reactions will limit the maximum applied gate voltage to values far below those needed to reach the high densities at which gate-induced superconductivity is present, in agreement with the gate voltage values reported in the above mention experiments ( $\approx 1 \text{ V}$ ).

#### S4. Ionic-gate spectroscopy measurement of the band gap of 2L-WSe<sub>2</sub>

In the main text we demonstrate the possibility to perform ionic-gate spectroscopy using LICGC gates, by measuring the single particle band gap of monlayer WSe<sub>2</sub> directly from the ambipolar transport curves of the transistors (see Fig. 4c). In this section we show the results of ionic-gate spectroscopy measurements performed on a 2L-WSe<sub>2</sub> LICGC-gated FET, as evidence of the reliability of the technique. The high-quality ambipolar transfer curve (four-probe conductivity  $\sigma_{4\text{p}}$ -vs- $V_{\text{Ref}}$ ) of a 2L-WSe<sub>2</sub> LICGC-gated FET (which contains a SiO<sub>2</sub> passivation layer) is shown in Fig. S5. As discuss elsewhere [12], the band gap of 2L-WSe<sub>2</sub> can be extracted as  $\Delta_{2\text{LWSe}_2} = e(V_{\text{Th}}^e - V_{\text{Th}}^h)$ , where  $V_{\text{Th}}^e$  and  $V_{\text{Th}}^h$  are the threshold voltages for electron and hole conduction, respectively. Extracting the value of  $V_{\text{Th}}^e$  and  $V_{\text{Th}}^h$  by extrapolating  $\sigma_{4\text{p}}$  to 0 S (as shown by the black-dashed lines in Fig. S5 for the sweep up curve) results in  $\Delta_{2\text{LWSe}_2} = 1.63 \pm 0.06 \text{ eV}$  (where the error is given by the different values obtained from multiple up-

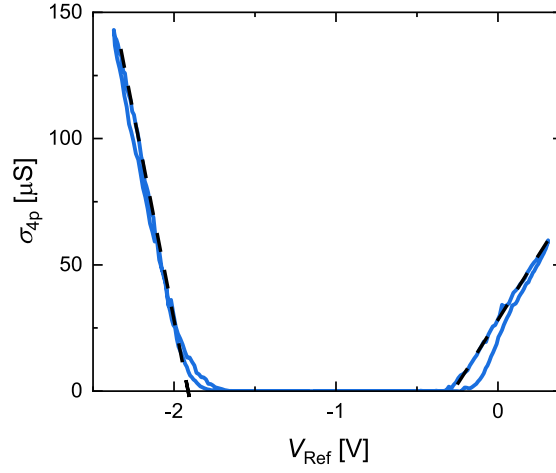

Figure S5: High-quality transistor characteristics of a 2L-WSe<sub>2</sub> LICGC-gated FETs realized with a SiO<sub>2</sub> passivation layer at the LICGC/Pt interface. The band gap of 2L-WSe<sub>2</sub> is measured directly from the ambipolar transfer (four-probe conductivity  $\sigma_{4p}$ -vs-reference potential  $V_{\text{Ref}}$ ) curve. The black-dashed lines represent the extrapolation of the linear regime to  $\sigma_{4p} = 0$  S (sweep up) used to extract the threshold voltages.

sweep and down-sweep curves), in good agreement with measurements performed with ionic-liquid gated FETs [12].

### S5. Transistor characteristics of the 3L-MoS<sub>2</sub> LICGC-gated FET used to investigate gate-induced superconductivity

An important result reached in the main text is the possibility to use LICGC gates to accumulate the high carrier densities ( $10^{14} \text{ cm}^{-2}$ ) needed to gate-induce superconductivity [13–19]. In this section we show the room temperature electron transistor characteristics of the 3L-MoS<sub>2</sub> LICGC-gated FET where gate-induced superconductivity was observed (the transistor characteristics were measured after the observation of superconductivity). The transfer curves (source-drain current  $I_{\text{SD}}$ -vs- $V_{\text{G}}$ ) shown in Fig. S6a

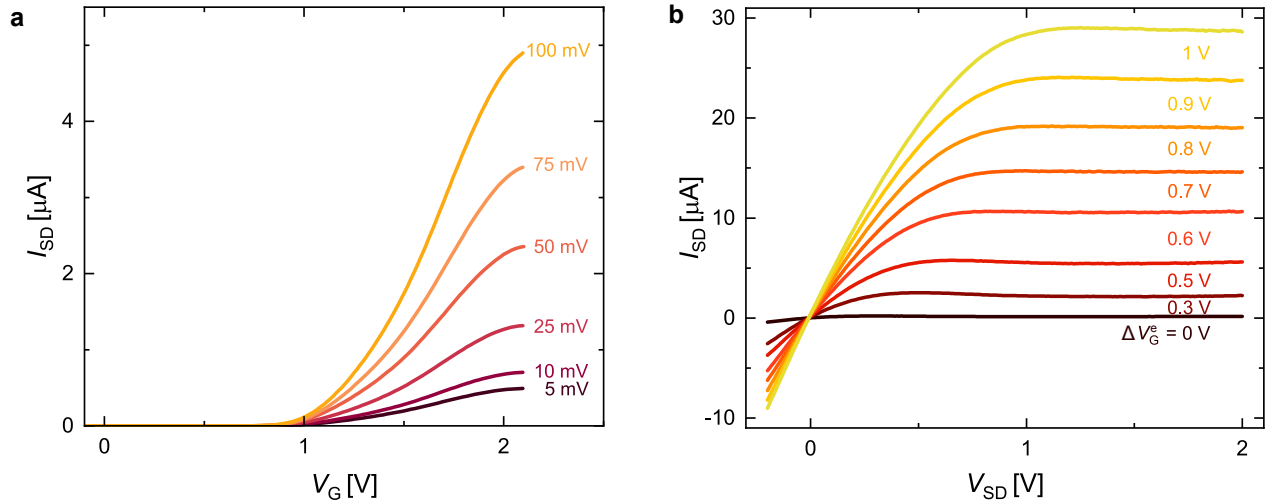

Figure S6: High-quality transistor characteristics of a 3L-MoS<sub>2</sub> LICGC-gated FET realized with a SiO<sub>2</sub> passivation layer in between the LICGC and the Pt electrodes, in which gate-induced superconductivity is seen at low-temperature. **a)** Transfer curves (source-drain current  $I_{\text{SD}}$  as a function of gate voltage  $V_{\text{G}}$ ) measured at different source-drain bias  $V_{\text{SD}}$ . **b)** Output ( $I_{\text{SD}}$ -vs- $V_{\text{SD}}$ ) curves measured at different values of  $\Delta V_{\text{G}}^e = V_{\text{G}} - V_{\text{Th}}^e$  ( $V_{\text{Th}}^e = 1.1$  V is the electron threshold voltage; this value differs from the 1.5 V observed during the investigation of superconductivity due to the effect of bias stress present during the realization of subsequent room-temperature Hall measurements).

for multiple source-drain voltages  $V_{SD}$ , exhibit a behaviour typically found in high-quality  $\text{MoS}_2$  ionic-gated FETs [20–23]. At low bias past the sub-threshold regime the current in the device increases linearly with gate voltage before saturating at higher applied gate voltage. The saturation (typically reached  $\approx 10^{14} \text{ cm}^{-2}$ ) signals the population of a second conduction band [24], which has been shown to be a requirement for the observation of superconductivity [19, 25]. The high-quality of the device is also showcased by the output ( $I_{SD}$ -vs- $V_{SD}$ ) curves shown in Fig. S6b, which exhibit textbook behaviour; at low  $V_{SD}$ ,  $I_{SD}$  increases linearly followed by the pinch-off of the channel at  $V_{SD} = V_G^e$ , after which  $I_{SD}$  saturates with the saturation current increasing for larger values of  $V_G^e$ .

### S6. High-quality transistor characteristics of a 2L-WSe<sub>2</sub> FET fabricated with the LASPT galss-ceramic

All other results presented in this work, i.e., the possibility to reach high carrier densities, perform ionic-gate spectroscopy and gate-induced superconductivity, were demonstrated in FETs fabricated with the AG-01 glass-ceramics. For comparison, here we show measurements performed on a 2L-WSe<sub>2</sub> FET device fabricated using a LASPT glass-ceramic with a  $\text{SiO}_2$  passivation layer. The high-quality transistor characteristics (Fig. S7) of the device, which show no signatures of parasitic effects (absence of electron transport and leakage current peaks caused by faradic reactions), demonstrate that the addition of a passivation layer constitutes a robust strategy to avoid the spurious effects of electrochemical reactions.

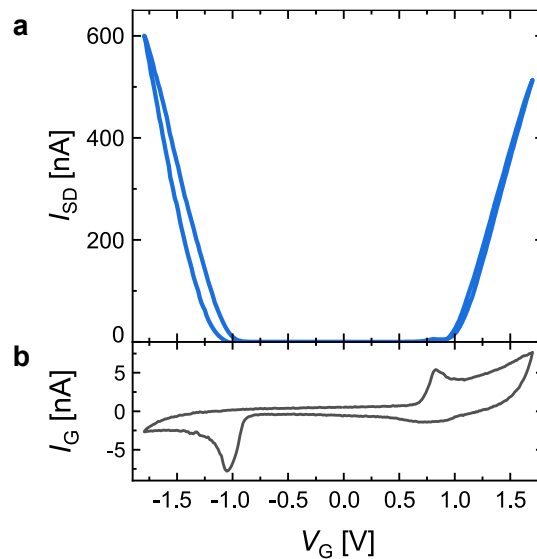

Figure S7: High-quality transistor characteristics of a LASPT gated 2L-WSe<sub>2</sub> FETs with a  $\text{SiO}_2$  passivation layer at the LICGC/Pt interface. **a)** Source-drain current  $I_{SD}$  as a function of gate voltage  $V_G$ . ( $V_{SD} = 50 \text{ mV}$ ) **b)** Leakage current  $I_G$ -vs- $V_G$ . The two peaks present in the curve are caused by the onset of charge accumulation [26], and not by chemical reactions (see discussion in main text and the evolution of the leakage current peaks in Figs. S4c, f, i and l).

## References

- [1] N. Elgrishi, K. J. Rountree, B. D. McCarthy, E. S. Rountree, T. T. Eisenhart, J. L. Dempsey, *Journal of chemical education* **2018**, *95*, 2 197.
- [2] J. Liu, J. Wang, C. Xu, H. Jiang, C. Li, L. Zhang, J. Lin, Z. X. Shen, *Advanced science* **2018**, *5*, 1 1700322.
- [3] A. J. Bard, L. R. Faulkner, *Electrochemical methods: fundamentals and applications*, John Wiley & Sons, **2001**.

- 
- [4] J. Wang, J. Polleux, J. Lim, B. Dunn, *The Journal of Physical Chemistry C* **2007**, *111*, 40 14925.
- [5] Y. Amiki, F. Sagane, K. Yamamoto, T. Hirayama, M. Sudoh, M. Motoyama, Y. Iriyama, *Journal of power sources* **2013**, *241* 583.
- [6] K. Yamamoto, Y. Iriyama, T. Hirayama, *Microscopy* **2017**, *66*, 1 50.
- [7] S. Russo, M. Craciun, M. Yamamoto, S. Tarucha, A. Morpurgo, *New Journal of Physics* **2009**, *11*, 9 095018.
- [8] B. E. Conway, *Journal of the Electrochemical Society* **1991**, *138*, 6 1539.
- [9] C. Sandford, M. A. Edwards, K. J. Klunder, D. P. Hickey, M. Li, K. Barman, M. S. Sigman, H. S. White, S. D. Minter, *Chemical science* **2019**, *10*, 26 6404.
- [10] M. H. Alam, Z. Xu, S. Chowdhury, Z. Jiang, D. Taneja, S. K. Banerjee, K. Lai, M. H. Braga, D. Akinwande, *Nature communications* **2020**, *11*, 1 1.
- [11] M. H. Alam, S. Chowdhury, A. Roy, M. H. Braga, S. K. Banerjee, D. Akinwande, *Physical Review Materials* **2021**, *5*, 5 054003.
- [12] I. Gutiérrez-Lezama, N. Ubrig, E. Ponomarev, A. F. Morpurgo, *Nature Reviews Physics* **2021**, *3*, 7 508.
- [13] J. Ye, S. Inoue, K. Kobayashi, Y. Kasahara, H. Yuan, H. Shimotani, Y. Iwasa, *Nature materials* **2010**, *9*, 2 125.
- [14] S. Jo, D. Costanzo, H. Berger, A. F. Morpurgo, *Nano letters* **2015**, *15*, 2 1197.
- [15] W. Shi, J. Ye, Y. Zhang, R. Suzuki, M. Yoshida, J. Miyazaki, N. Inoue, Y. Saito, Y. Iwasa, *Scientific reports* **2015**, *5*, 1 1.
- [16] D. Costanzo, S. Jo, H. Berger, A. F. Morpurgo, *Nature nanotechnology* **2016**, *11*, 4 339.
- [17] D. Costanzo, H. Zhang, B. A. Reddy, H. Berger, A. F. Morpurgo, *Nature nanotechnology* **2018**, *13*, 6 483.
- [18] J. Lu, O. Zheliuk, Q. Chen, I. Leermakers, N. E. Hussey, U. Zeitler, J. Ye, *Proceedings of the National Academy of Sciences* **2018**, *115*, 14 3551.
- [19] E. Piatti, D. De Fazio, D. Daghero, S. R. Tamalampudi, D. Yoon, A. C. Ferrari, R. S. Gonnelli, *Nano letters* **2018**, *18*, 8 4821.
- [20] Y. Zhang, J. Ye, Y. Matsushashi, Y. Iwasa, *Nano letters* **2012**, *12*, 3 1136.
- [21] J. Ye, Y. Zhang, Y. Iwasa, *MRS Online Proceedings Library (OPL)* **2013**, *1549* 73.
- [22] M. M. Perera, M.-W. Lin, H.-J. Chuang, B. P. Chamlagain, C. Wang, X. Tan, M. M.-C. Cheng, D. Tománek, Z. Zhou, *ACS nano* **2013**, *7*, 5 4449.
- [23] E. Ponomarev, I. Gutiérrez-Lezama, N. Ubrig, A. F. Morpurgo, *Nano letters* **2015**, *15*, 12 8289.
- [24] H. Zhang, C. Berthod, H. Berger, T. Giamarchi, A. F. Morpurgo, *Nano Letters* **2019**, *19*, 12 8836.
- [25] T. Sohler, E. Ponomarev, M. Gibertini, H. Berger, N. Marzari, N. Ubrig, A. F. Morpurgo, *Physical Review X* **2019**, *9*, 3 031019.
- [26] D. Braga, I. Gutiérrez-Lezama, H. Berger, A. F. Morpurgo, *Nano letters* **2012**, *12*, 10 5218.
